# Supplementary material for: Descriptors for Electrolyte-Renormalized Oxidative Stability of Solvents in Lithium-ion Batteries
Source: arXiv:1908.03285 source file (2019-08-08)
Supplement: Supplementary file 1 [file SI.pdf]

# Supporting Information for "Descriptors for Electrolyte-Renormalized Oxidative Stability of Solvents in Lithium-ion Batteries"

Vikram Pande and Venkatasubramanian Viswanathan*

*Department of Mechanical Engineering, Carnegie Mellon University, Pittsburgh, Pennsylvania 15213, USA*

E-mail: venkvis@cmu.edu

Table 1: Comparison of experimentally determined and DFT calculated Ionization Potentials for 34 solvents.

| Solvent | Experimental IP (eV) | DFT Calculated IP (eV) |
|---|---|---|
| 1,2-dichloroethane | 11.04 | 10.34 |
| 1,2-dimethoxyethane | 9.30 | 8.91 |
| 2-methyl-2-propanol | 9.90 | 9.57 |
| 2-propanol | 10.17 | 9.94 |
| acetic acid | 10.65 | 10.78 |
| acetonitrile | 12.20 | 12.17 |
| benzene | 9.24 | 9.40 |
| benzonitrile | 9.70 | 9.63 |
| benzyl alcohol | 8.30 | 8.81 |
| butanol | 9.99 | 9.48 |
| dichloromethane | 11.32 | 10.73 |
| diethyl ether | 9.51 | 9.40 |
| diethylamine | 7.85 | 8.20 |
| dimethyl sulfoxide | 9.10 | 8.86 |
| dioxane | 9.19 | 8.63 |
| ethanol | 10.43 | 10.21 |
| ethyl acetate | 10.01 | 10.08 |
| formamide | 10.16 | 10.64 |
| formic acid | 11.33 | 11.75 |
| heptane | 9.93 | 9.36 |
| hexane | 10.13 | 9.58 |
| Methanol | 10.85 | 10.88 |
| methyl acetate | 10.25 | 10.40 |
| N-methylformamide | 9.83 | 9.89 |
| nitrobenzene | 9.86 | 9.79 |
| nitromethane | 11.08 | 11.17 |
| propanol | 10.18 | 9.71 |
| pyridine | 9.25 | 9.31 |
| sulfolane | 9.80 | 9.69 |
| tetrahydrofuran | 9.38 | 9.26 |
| trichloromethane | 11.37 | 10.72 |
| triethylamine | 7.50 | 7.63 |
| water | 12.62 | 12.67 |

Table 2: Solvent HOMO renormalization for 41 solvent-salt complexes. The renormalization was calculated w.r.t the solvent and hence no values were given for the cases where salt got oxidized, represented by A and S,A in column 3.

| Solvent | Salt | Oxidized specie | Solvent HOMO renormalization (eV) |
|---|---|---|---|
| TEA | $LiCF_3SO_3$ | S | 0.42 |
| TEA | $LiNO_3$ | S | 0.53 |
| TEA | $LiPF_6$ | S | 0.30 |
| TEA | LiTFSI | S | 0.54 |
| TEA | LiOCN | S | 0.80 |
| TEA | $LiClO_4$ | S | 0.45 |
| TEA | LiSCN | S,A | - |
| DME | $LiCF_3SO_3$ | S | 0.77 |
| DME | $LiNO_3$ | S | 0.93 |
| DME | $LiPF_6$ | S | 0.49 |
| DME | LiTFSI | S | 0.99 |
| DME | LiOCN | S | 1.35 |
| DME | $LiClO_4$ | S | 0.79 |
| DME | LiSCN | S,A | - |
| DMSO | $LiCF_3SO_3$ | S | 1.27 |
| DMSO | $LiNO_3$ | S | 1.01 |
| DMSO | $LiPF_6$ | S | 0.54 |
| DMSO | LiTFSI | S | 0.88 |
| DMSO | LiOCN | S | 1.31 |
| DMSO | $LiClO_4$ | S | 0.74 |
| DMSO | LiSCN | S,A | - |
| NMF | $LiCF_3SO_3$ | S | 1.34 |
| NMF | $LiNO_3$ | S | 1.51 |
| NMF | $LiPF_6$ | S | 0.70 |
| NMF | LiTFSI | S | 1.50 |
| NMF | LiOCN | S | 1.73 |
| NMF | $LiClO_4$ | S | 1.17 |
| NMF | LiSCN | A | - |
| Methanol | $LiCF_3SO_3$ | S | 1.88 |
| Methanol | $LiNO_3$ | S,A | - |
| Methanol | $LiPF_6$ | S | 1.14 |
| Methanol | LiTFSI | A | - |
| Methanol | LiOCN | A | - |
| Methanol | $LiClO_4$ | S,A | - |
| Ethanol | $LiCF_3SO_3$ | S | 1.71 |
| Ethanol | $LiNO_3$ | S | 1.66 |
| Ethanol | $LiPF_6$ | S | 0.92 |
| Ethanol | LiTFSI | S | 1.66 |
| Ethanol | LiOCN | S | 2.48 |
| Ethanol | $LiClO_4$ | S | 1.52 |
